# Supplementary material for: Multi-Sensor Event Detection using Shape Histograms
Source: arXiv:1408.3733 source file (2014-08-16)
Supplement: Supplementary file 1 [file appendix.tex]

\begin{table}[!h]
\centering
\caption{Dataset Summary}
\label{Tb_DataDesc}
\begin{tabular}{|p{1.6cm}|p{4.5cm}|p{1.8cm}|}
\hline
Dataset Name & Data Description & Reference\\
\hline
Coffee & It consists of spectrograph samples of two widely produced coffee types. & \cite{Lines:2012} \\
\hline
Face (four) & It is a collection of pseudo time series data converted by head profile of four different individuals making different expressions such as talking, smiling, laughing, frowning etc. In this context, time-series represent the local angle of its perimeter trace starting from the neck area. Objective is to classify the head pose. & \cite{Face_dataset} \\
\hline
Wafer & Wafer dataset include measurements of a vacuum-chamber sensor during the etch process of silicon wafer manufacture. After the processing, each wafer is classified as normal or abnormal. The classification objective here was to identify the data-streams corresponding to normal/abnormal wafers. & \cite{Wei:2006,dataset:Keogg}\\
\hline
Sony-AIBORobot Surface \newline \newline Sony-AIBORobot SurfaceII & This dataset contains accelerometer data-streams of a SONY AIBO Robot dog walking on two different surfaces: carpet and cement. Only X-axis readings have been considered where each data-stream correspond to one robot walk having 70 / 65 measurements. The objective to identify the surface of the walk; here, noisy data and small training set poses complex 2-category classification problem. & \cite{dataset:Keogg} \\
\hline
Beef & The dataset contains 60 data-streams of spectrogram measurements having pure and adulterated beef with varying degrees of offal. Each data-stream is 470 values long belonging to one of the five distinct categories based on the quality. Classification objective is identification of the quality. & \cite{BagnallDHL12}\\
\hline
\end{tabular}
\end{table}

\begin{table}[!h]
\centering
\caption{Dataset Summary}
\label{Tb_DataDesc}
\begin{tabular}{|p{1.6cm}|p{4.5cm}|p{1.8cm}|}
\hline
Dataset Name & Data Description & Reference\\
\hline
\hline
OliveOil & Similar to Beef dataset, this dataset contains 60 data-streams of spectrogram measurements of Oliveoil belonging to four classes. Here, a class denote the geographic origin of the olive oil. & \cite{BagnallDHL12}\\
\hline
Trace & This dataset is a subset of synthetic dataset designed to simulate the instrumentation failures in a nuclear power plant. It is compiled with only second feature of class 2 and 6, and second feature of class 3 and 7 \cite{RatanamahatanaK04} & \cite{Roverso00,dataset:Keogg} \\
\hline
ECG & Electrocardiogram (ECG) dataset contains measurements of cardiac electrical activity as recorded
from electrodes at various locations on the body. Each data-stream in the dataset has the measurements recorded by one electrode during one heartbeat. All of the data-streams have been normalized to vector having 96 values, and have a label of normal or abnormal as annotated by domain expert. & \cite{Olszewski:2001}\\
\hline
Lightning-2 & & \cite{Lin:2007,4634188} \\
\hline
Lightning-7 &  & \cite{libsvmDE02a} \\
\hline
Italy-Power-Demand & describing per day, average per hour power demand in Italy from the period of January to June. Here, the classification objective is to predict the quarter (January-March, April-June) of the recorded power-demand time-series.
In particular, the dataset poses unique challenge, as in the same class, i.e., quarter, power demand varies significantly from weekdays to holidays. 
Also, similarity in weather pattern in continuous months would influence similar power demand pattern in March and April. & \cite{Lines:2012} \\
\hline
\end{tabular}
\end{table}

\begin{table}[!h]
\centering
\caption{Dataset Summary}
\label{Tb_DataDesc}
\begin{tabular}{|p{1.6cm}|p{4.5cm}|p{1.8cm}|}
\hline
Dataset Name & Data Description & Reference\\
\hline
Medical-Images & The MedicalImages dataset poses 10-category classification problem of data-streams having 99 values. Data-streams are the pixel intesity histograms of medical images with each class represent different human body region. In object recognition research, several methods have been proposed for this particular problem. & \cite{dataset:Keogg} \\
\hline 
FacesUCR & The FacesUCR dataset is a collection of the instances of 14 face images transformed into time-series. The time-series data represents the local angle of the perimeter trace of face images starting from the neck. The collection has 2250 images from 14 individuals under different conditions including variety of expressions, and with/without eyeglasses. The problem is particularly complex because of variations in head angle, expressions with some wearing eyeglasses. & \cite{dataset:Keogg}\\
\hline
Diatom-Size-Reduction & This dataset has a collection of diatom images in pseudo time series. The objective of this dataset is to explore the distribution of shapes and valve face features of diatoms in morphospace.  & \cite{dataset:Keogg}\\
\hline
Chlorine-Concen-tration & Chlorine concentration dataset consists of data-streams having the measurement of chlorine concentration level in a water network . The measurements are captured at 166 pipe junctions generating equally long time-series.  & \cite{Li:2009} \\
\hline
Adiac & Adiac dataset consists of 781 daitom contour-streams of 37 taxon types, i.e, classes. Each taxon type, signifies a species or variety, has at least 20 representatives. & \cite{Adiac_2005}\\
\hline
Synthetic-Control & This dataset contains 600 examples of synthetically generated control charts. A control pattern is a time-series showing the machine parameter variation with respect to time. There are six different classes of control charts generated by six different equations. & \cite{Alcock99} \\
\hline
SwedishLeaf & This dataset consists of 1125 Swedish leaf images converted in the time-series form by measuring the distance of contour points of the image with respect to its centroid & \cite{Xi:2006}\\ 
\hline
\end{tabular}
\end{table}

\begin{table}[!h]
\centering
\caption{Dataset Summary}
\label{Tb_DataDesc}
\begin{tabular}{|p{1.6cm}|p{4.5cm}|p{1.8cm}|}
\hline
Dataset Name & Data Description & Reference\\
\hline
Symbols & Each instance in this dataset is a data-series generated by X or Y-axis trace of the freehand drawing of a given symbol by a volunteer \cite{dataset:Keogg}. Each data-series has 398 values. There are 3 symbols, generating 6 different classes by individual labelling of X, and Y-axis traces. This poses a complex challenge for classification, because, even for different symbols, individual traces exhibit significant similarity. & \cite{dataset:Keogg}\\
\hline 
TwoLead-ECG & This dataset poses heartbeat classification task in two classes, i.e., normal/abnormal. Classification on this dataset is challenging task because of subtle distinctions between samples from two classes, and very small training set. & \cite{Ye:2009,Lines:2012} \\
\hline
MoteStrain & This data is a collection the month long recording of 48 Mote sensors installed in a lab environment. In this dataset, we have recording from two different sensors. The streams are in z-normalized form having vector of 84 values. In particular, streams have large inter-class variations with many zeros because of drop-outs. & \cite{Ye:2009,Lines:2012}\\
\hline
ECG-FiveDays & This dataset has a collection of ECG data series of a single patient recorded on the duration of five days. Each data series is annotated as either normal, or abnormal. & \cite{Ye:2009}\\
\hline
Gun-point & This dataset \cite{RatanamahatanaK04} consists of hand-motion patterns of an actor depicting gun drawing action from a hip mounted holster, gun-pointing at the target for approximately one second and returning to normal state. 
The dataset has been widely applied for evaluation of many frameworks for time-series analysis. 
Patterns in the dataset describe two categories representing real and fake gun pulling action. & \cite{Ye:2009}\\
\hline
\end{tabular}
\end{table}
